# Supplementary material for: Bottleneck Transformers for Visual Recognition
Source: arXiv:2101.11605 source file (2021-08-02)
Supplement: Supplementary file 1 [file appendix.tex]

\begin{appendix}
\section{Appendix}

\subsection{Code for the BoT block}

We provide the exact code used for implementing the Multi-Head Self-Attention (MHSA) in 2D with relative-position encodings as well as the implementation of BoT block in this \texttt{gist} link: \url{https://gist.github.com/aravindsrinivas/56359b79f0ce4449bcb04ab4b56a57a2}.

\subsection{Implementation: COCO Instance Segmentation and Object Detection}

Our implementation is based on the Cloud TPU Detection codebase - \url{https://github.com/tensorflow/tpu/tree/master/models/official/detection}. Our canonical setting uses the following hyperparameters which are updated in \texttt{configs/maskrcnn\_config.py}: 

\begin{itemize}
    \item \texttt{output\_size} of $1024 \times 1024$.
    \item \texttt{aug\_scale\_min=0.8,aug\_scale\_max=1.25}
    \item \texttt{mrcnn\_head:num\_convs=4,
num\_filters=256,mask\_target\_size=28}
    \item \texttt{frcnn\_head:num\_convs=4,
num\_filters=256,fc\_dims=1024,
num\_fcs=1}
    \item \texttt{rpn\_head:min\_level=2,
max\_level=6,
anchors\_per\_location=3,
num\_convs=2,num\_filters=256}
    \item \texttt{fpn:min\_level=2,max\_level=6}
    \item \texttt{anchor:
num\_scales=1,anchor\_size=8,
min\_level=2,max\_level=6}
\end{itemize}

For all experiments, we use L2 weight decay of $4e-5$, sync-batch-norm with momentum 0.997 and epsilon 1e-4. We use batch norm in the backbone, FPN, RPN head, FRCNN head and MRCNN head. We initialize backbone weights with pre-trained ImageNet checkpoints and fine-tune all the weights (including the batch-norm parameters) as specified in MoCo~\cite{he2020momentum}.

Table \ref{tab:schedule} presents the hyperparameters for models that we train with batch size 64 on 8 TPU-v3 cores (equivalent to DGX-1) which applies to most of our models, in particular, all the models that we train with image size $1024 \times 1024$.

\begin{table}[!ht]\centering
\small
\setlength\tabcolsep{2.0pt}
\begin{tabular}{l|c|c|c}
\Xhline{1.0pt}
\text{Type}  & \text{Epochs} & \text{Train Steps} & \text{LR Schedule} \\[2pt]
\Xhline{1.0pt}
1x & 12 & 22.5k & [15k, 17.5k] \\
2x & 24 & 45k &  [37.5k, 40k] \\
3x & 36 & 67.5k & [60k, 65k] \\
6x & 72 & 135k & [120k, 130k] \\
\hline
\Xhline{1.0pt}
\end{tabular}
\vspace*{-0mm}
\caption{Learning Rate Schedules for the 1x, 2x, 3x and 6x settings for models trained with global batch size of 64, 8 TPU-v3 cores, 16 GB HBM per cores, learning rate 0.1 with schedule [0.01, 0.001]. The learning rate is initially warmed up for 500 warmup steps from 0.0067.}
\label{tab:schedule}
\vspace{-2mm}
\end{table}

For models that do not fit with batch size of 8 per core (for example, the ones that train with $1280\times 1280$), we train with a global batch size of 128 on 32 TPU-v3 cores (4 images per core). The 6x schedule for these models that train with 32 cores corresponds to training with 67.5k steps (since batch size 128 is double 64), with [60k, 65k] learning rate schedule. The learning rate is 0.15 with schedule [0.015, 0.0015] with 500 warmup steps started from 0.0067. 

For the model that achieves best results (44.4\% mask AP) with ResNet-200 backbone and BoTNet structure for blockgroup \texttt{c5}, we use 8 convolutions in the MRCC head.

For our object detection experiments, we just turned off the mask branch by setting the \texttt{include\_mask} flag as \texttt{False} and \texttt{eval\_type} as \texttt{box} instead of \texttt{box\_and\_mask}.

\subsection{BoTNet improves over ResNet for Object Detection}
\label{sec:frcnn}

Does BoTNet improve upon ResNet for the task of object detection as well? We verify this through experiments with the Faster R-CNN framework (Table \ref{tab:faster}). %For Tables \ref{tab:faster}, we use the canonical setting\footnote{36 epochs, $1024\times 1024$ images, $[0.8,1.25]$ jitter.}. 
We observe that BoTNet indeed improves over ResNet significantly. BoT R50 improves upon R50 by a {significant margin of + 1.6\%} \apbbox{S} (\apbbox{} for {small objects}). %while BoT R101 improves upon R101 on AP$_S$ by {\bf 3.7\%}. 
These results suggest that {\it self-attention has a big effect in detecting small objects} which is considered to be an important and hard problem for deploying object detection systems in the real world. This result is in contrast with DETR~\cite{carion2020end} which observes a big improvement on large objects but not on small objects. We believe that introducing self-attention in the backbone architecture might help fix the lack of gains on small objects in DETR. Finally, we study if larger images would further benefit BoTNet for object detection. Using a multi-scale jitter of $[0.1, 2.0]$ with 72 epoch training and image size of $1280 \times 1280$, we see that BoT R152 achieves a strong performance of {\bf 48.4\%} \apbbox{}.

\begin{table}[ht]\centering
 \small
 \setlength\tabcolsep{2.5pt}
 \begin{tabular}{l|c|c|c}
 \Xhline{1.0pt}
  \text{Backbone}  &   \apbbox{} & \apbbox{S} & \apbbox{L} \\[2pt]
  %\text{Backbone}  & \texttt{res} &  AP & AP$_{50}$ & AP$_{75}$ & AP$_{S}$ & AP$_{M}$ & AP$_{L}$ \\[2pt]
 \Xhline{1.0pt}

R50  & 41.5 &	24.9 &	54.3 \\
BoT50  & 43.1 (\textcolor{ForestGreen}{+ {\bf 1.6}}) &	27.6 (\textcolor{ForestGreen}{+ {\bf 2.7}}) &	55.7 (\textcolor{ForestGreen}{+ {\bf 1.3}}) \\
\hline
R101 & 42.4 & 	24.5 &	55.0 \\
BoT101  & 44.3 (\textcolor{ForestGreen}{+ {\bf 1.9}}) & 26.5 (\textcolor{ForestGreen}{+ {\bf 2.0}}) &	57.5 (\textcolor{ForestGreen}{+ {\bf 2.5}}) \\
\hline
R152 & 45.1 &	30.1 &	56.6 \\
BoT152 & {\bf 48.4} (\textcolor{ForestGreen}{+ {\bf 3.3}}) &	{\bf 32.7} (\textcolor{ForestGreen}{+ {\bf 2.6}}) 	 &  {\bf 60.6} (\textcolor{ForestGreen}{+ {\bf 4.0}}) \\

\Xhline{1.0pt}
\end{tabular}
\vspace*{-0mm}
\caption{{BoTNet for Faster R-CNN:} The first four rows are trained for 36 epochs, jitter $\left[0.8,1.25\right]$, image size $1024\times 1024$. Final two rows are trained for 72 epochs with $1280\times1280$ image size, jitter $\left[0.1,2.0\right]$ using \texttt{v3-32} Cloud TPU.}
%\caption{\textbf{BoTNet and ResNet for Faster R-CNN:} Both BoT R50 and BoT R101 show significant improvement over R50 and R101 on \apbbox{} ({\bf + 1.8\%} and {\bf + 2.3\%} respectively). The gains on AP$_S$ (small objects) is remarkable: {\bf + 4.3\%} and {\bf + 3.7\%} for BoT R50 and BoT R101 respectively.}
\label{tab:faster}
\vspace{-2mm}
\end{table}

%%%%%%%%%%%%%%%%
\subsection{Why replace all three \texttt{c5} spatial convolutions?}
\label{sec:configs}

\begin{figure}[ht]%
    \centering
    \includegraphics[scale=0.4]{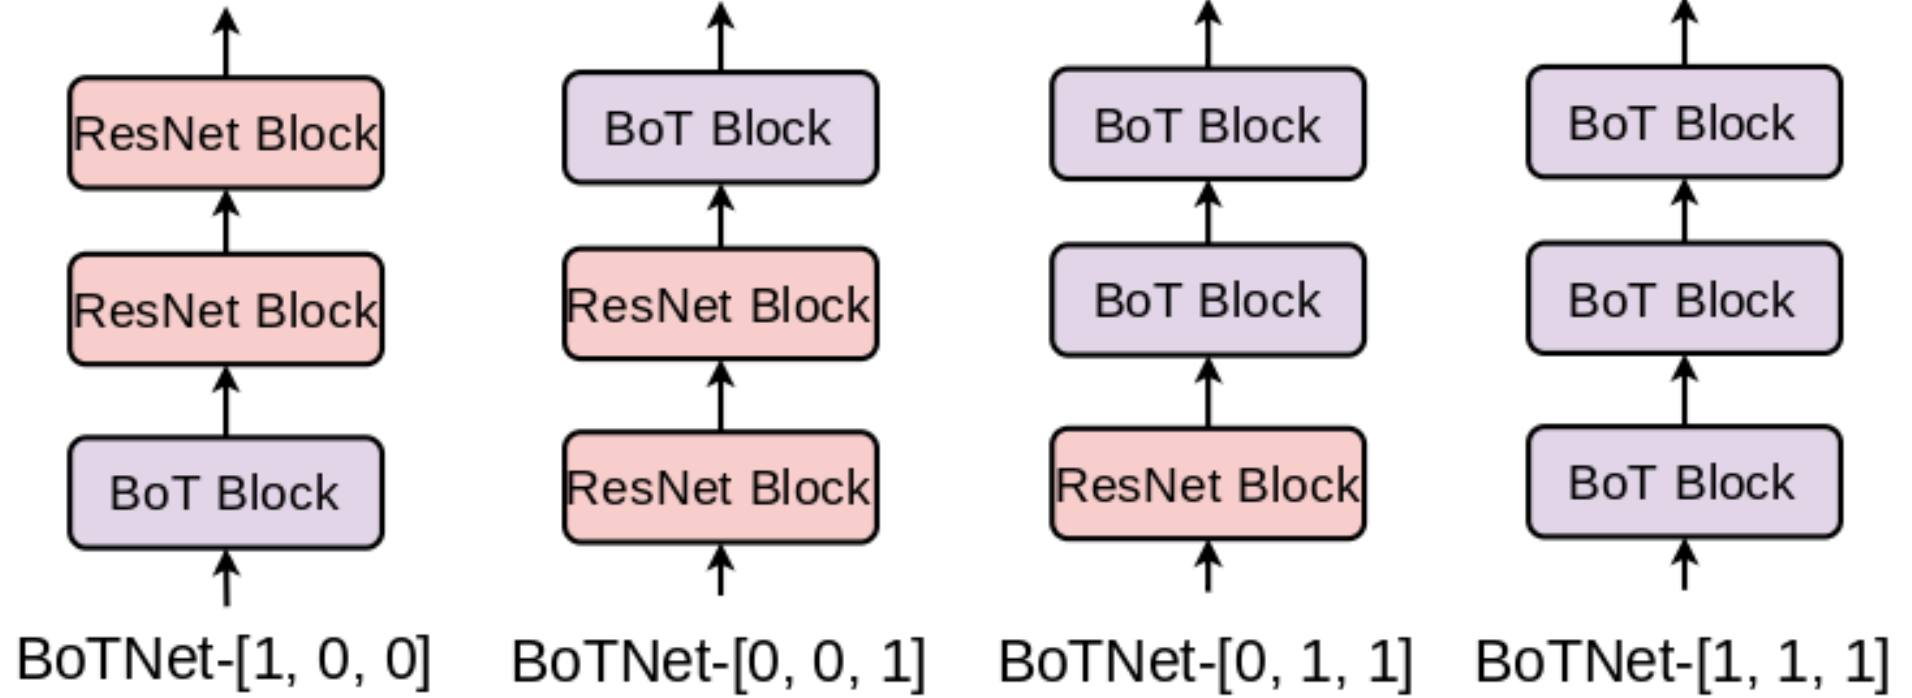}
    \caption{Replacement configs for BoTNet in the \texttt{c5} blockgroup of a ResNet}%
    \label{fig:configs}%
\end{figure}

\begin{table*}[!ht]\centering
\small
\setlength\tabcolsep{3.5pt}
\begin{tabular}{l|c|c|ccc|ccc}
\Xhline{1.0pt}

\text{Backbone}  & \texttt{c5-attn.} & \texttt{TC Time} & {\apbbox{}} & \apbbox{S} & \apbbox{L} &  {\apmask{}} &  \apmask{S} & \apmask{L} \\[2pt]

\Xhline{1.0pt}

R50 &  \texttt{[0,0,0]} & 786.5 & 42.1  & 22.5	& 59.1 & 37.7 & 18.3	& 54.9 \\
BoT 50 & \texttt{[0,0,1]} & 813.7 & 43.4 (\textcolor{ForestGreen}{+ {\bf  1.3}}) & 23.7 (\textcolor{ForestGreen}{+ {\bf    1.2}}) &		59.7 (\textcolor{ForestGreen}{+ {\bf    0.6}}) & 38.6 (\textcolor{ForestGreen}{+ {\bf  0.9}})  &	19.0 (\textcolor{ForestGreen}{+ {\bf    0.7}}) &	55.6 (\textcolor{ForestGreen}{+ { \bf  0.7}}) \\
BoT 50 & \texttt{[0,1,1]} & 843.87 & 43.4 (\textcolor{ForestGreen}{+ {\bf  1.3}}) & 24.0 (\textcolor{ForestGreen}{+ {\bf    1.5}})	 & 60.2 (\textcolor{ForestGreen}{+ {\bf    1.1}}) & 38.6 (\textcolor{ForestGreen}{+ {\bf  0.9}}) &	19.4 (\textcolor{ForestGreen}{+ {\bf    1.1}}) &	55.9 (\textcolor{ForestGreen}{+ {\bf    1.0}}) \\
BoT R50 & \texttt{[1,0,0]} & 983.2 & 43.7 (\textcolor{ForestGreen}{+ {\bf  1.6}}) & 23.9 (\textcolor{ForestGreen}{+ {\bf    1.4}}) & {60.6} (\textcolor{ForestGreen}{+ {\bf    1.5}}) & 38.9 (\textcolor{ForestGreen}{+ {\bf   1.2}})   &	 {19.3} (\textcolor{ForestGreen}{+ {\bf    1.0}}) & 55.9 (\textcolor{ForestGreen}{+ {\bf    1.0}}) \\
BoT 50 & \texttt{[1,1,1]} & 1032.7 & 43.6 (\textcolor{ForestGreen}{+ {\bf   1.5}}) & 25.1 (\textcolor{ForestGreen}{+ {\bf 2.6}})  &	59.4 ({+ { 0.3}}) &	38.9 (\textcolor{ForestGreen}{+ {\bf   1.2}})  &	20.7 (\textcolor{ForestGreen}{+ {\bf 2.4}}) &	55.5 (\textcolor{ForestGreen}{+ {\bf 0.6}}) \\
\hline
R101 & \texttt{[0,0,0]} & 928.7 & 43.3 (\textcolor{ForestGreen}{+ {\bf  1.2}}) & 24.2 (\textcolor{ForestGreen}{+ {\bf  1.7}})  & 60.7 (\textcolor{ForestGreen}{+ {\bf  1.6}}) & 38.4 (\textcolor{ForestGreen}{+ {\bf  0.7}})  & 19.6 (\textcolor{ForestGreen}{+ {\bf  1.3}})  & 56.8 (\textcolor{ForestGreen}{+ {\bf  1.9}}) \\
BoT101 & \texttt{[1,1,1]} & 1174.9 & 45.5 (\textcolor{ForestGreen}{+ {\bf 2.2}})	& 26.0 (\textcolor{ForestGreen}{+ {\bf 1.8}}) &	62.3  (\textcolor{ForestGreen}{+ {\bf 1.6}}) &	40.4 (\textcolor{ForestGreen}{+ {\bf 2.0}})		&		21.1  (\textcolor{ForestGreen}{+ {\bf 1.5}})	&	58.0  (\textcolor{ForestGreen}{+ {\bf 1.2}}) \\

\Xhline{1.0pt}

\Xhline{1.0pt}
\end{tabular}
\vspace*{-0mm}
\caption{{Ablation study on the replacement design in BoTNet:} All models are trained with the canonical config with image size $1024\times 1024$, jitter $\left[0.8, 1.25\right]$, 36 epochs. %We see that all designs have significant improvements over the baseline R50. 
TC Time refers to TPU-v3 Compute Step Time (in milliseconds) during training.}
\label{tab:placement}
\vspace{-2mm}
\end{table*}

\vspace{-2mm}

Is replacing all the 3 spatial convolutions in \texttt{c5} the {\it minimum effective} change or could it be simplified even further? We perform an ablation study on the replacement design in order to answer this question (Please refer to Table \ref{tab:placement}, Figure \ref{fig:configs}). The baseline R50 and BoT50 go by the notation \texttt{[0,0,0]} and \texttt{[1,1,1]} since the former does not replace anything while the latter replaces the spatial convolution in all three \texttt{c5} blocks. As mentioned already, the first replacement in \texttt{c5} operates on $64\times64$ feature map while the remaining two operate on $32\times 32$. We ablate for the configs: \texttt{[0,0,1]}, \texttt{[0,1,1]} and \texttt{[1,0,0]}. The first two configs test how useful is the replacement when performed only on the smaller $32\times 32$ featuremap(s) once and twice respectively, while the last tests how useful is the replacement when performed only on the larger $64 \times 64$ featuremap.

First, we see that in terms of aggregate measures such as \apbbox{} and \apmask{}, each of the configs for BoT50 is a strict improvement over R50, with similar performance. Config. \texttt{[1,0,0]} is closer to the performance of BoT50 (\texttt{[1,1,1]}) compared to the other configurations, however a difference of 0.2 \apbbox{} is within the noise typically observed in COCO experiments. It is indeed surprising that just a single self-attention replacement layer right at the end (\texttt{[0,0,1]}) provides a visible gain of 1.3 \apbbox{}. When contrasted with the performance of R101 (43.2 \apbbox{} and 38.4 \apmask{}), the config. \texttt{[0,0,1]} is very much competitive with 43.4 \apbbox{} and 38.6 \apmask{}, with more efficient compute steptime on the TPU (1.2x faster). Nevertheless, the gains on large objects for the \texttt{[0,0,1]} config (+ 0.6 \apbbox{L}) are not as significant as those in R101 (+ 1.6 \apbbox{L}).

Among the different configs for BoT50, we see that \texttt{[1,0,0]} and \texttt{[0,1,1]} are the best in terms of good performance on both small and large objects. Surprisingly, the actual BoTNet config (\texttt{[1,1,1]}) shows significant boost on small objects (2.6 \apbbox{S}), but does not show substantial gain on large objects, even relative to other ablation configs. We suspect this could be due to poor optimization and leave it for future work to carefully understand how self-attention affects the performance on small and large objects.

Based on these ablations, consider the question: is it better to replace convolutions with self-attention in \texttt{c5} (BoT50) vs stacking more convolution layers (R101)? An argument in favor of R101 is that the gains are clear on both small and large objects unlike BoT50 where the gains are much more on small objects. However, there does exist a BoT50 config that can strictly improve upon R101, ie the \texttt{[0,1,1]} config. It has similar properties to R101 (gain on both small and large objects), similar performance on aggregate measures like \apbbox{} and \apmask{}, with a more efficient compute steptime. Hence, we can affirmatively say that {\it self-attention replacement is more efficient than stacking convolutions}.

%One could also get the best of both worlds, stacking more convolutions as well as replacing the final convolutions with self-attention. We do observe that in BoT101 where we see significant boost on both \apbbox{S}, \apbbox{L}; and \apmask{S} and \apmask{L}.

\subsection{BoT block with stride}

The first block in the final block group \texttt{c5} of a ResNet runs the spatial $3\times3$ convolution with a stride 2 on a resolution that is 2x the height and width of the other two blocks in the group. Unlike spatial convolutional layers, the MHSA layers in BoT blocks do not implement striding. In fact, implementing strided self-attention without strided convolutions (both local and global) is an engineering challenge which we leave for future work. Our goal is to only use existing primitives. So, we adopt a very simple fix of using a local $2\times2$ Avg. Pooling with stride of 2 for implementing the spatial downsampling in the first BoT block. As noted in our ablation on placement of the attention (Section \ref{sec:configs}), we see that the self-attention in the first block is very useful for gain on small objects. At the same time, it involves running self-attention on a resolution of $64\times 64$, equivalent to 4096 tokens and $4096\times4096$ query-key matrix. We believe a well optimized strided attention implementation will drastically make this more efficient in future. The block is explained in Figure \ref{fig:strided}.

\begin{figure}[ht]
\centering
\includegraphics[scale=.35]{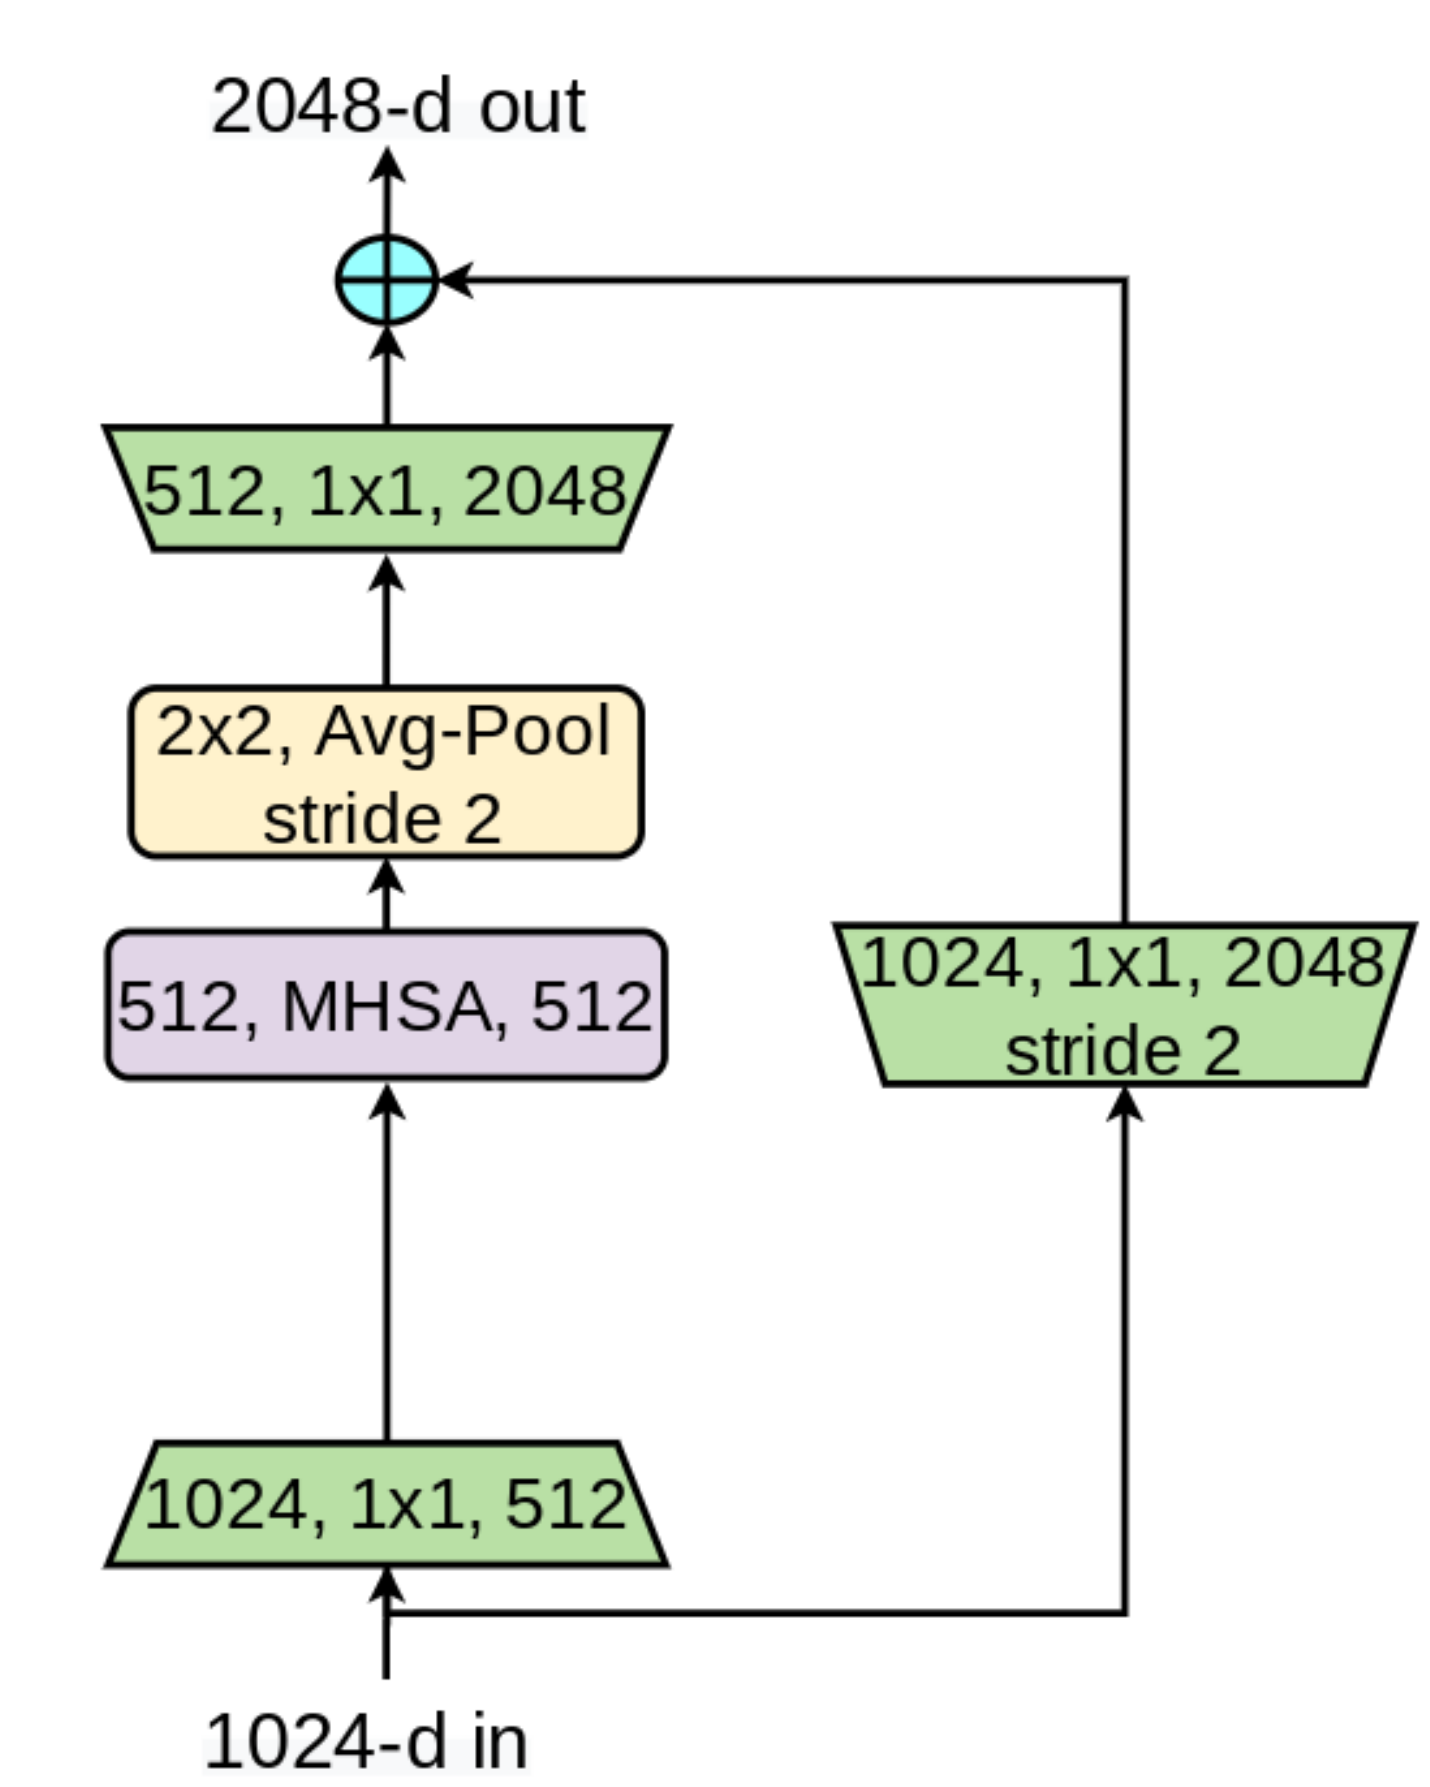}

\caption{BoT block with stride=2, implemented in the first block of the \texttt{c5} blockgroup in a BoT-ResNet. Since the incoming tensor has 1024 channels and has a stride of 16 with respect to input resolution, there is a projection shortcut with a strided $1\times1$ convolution. The self-attention operation in the MHSA is global and maintains the resolution. Therefore, we use local 2x2 Avg. Pooling with a stride 2 on top of it.}
\label{fig:strided}
\end{figure}

\subsection{BoTNet-S1}

\begin{figure}[H]%
    \centering
    \includegraphics[scale=0.4]{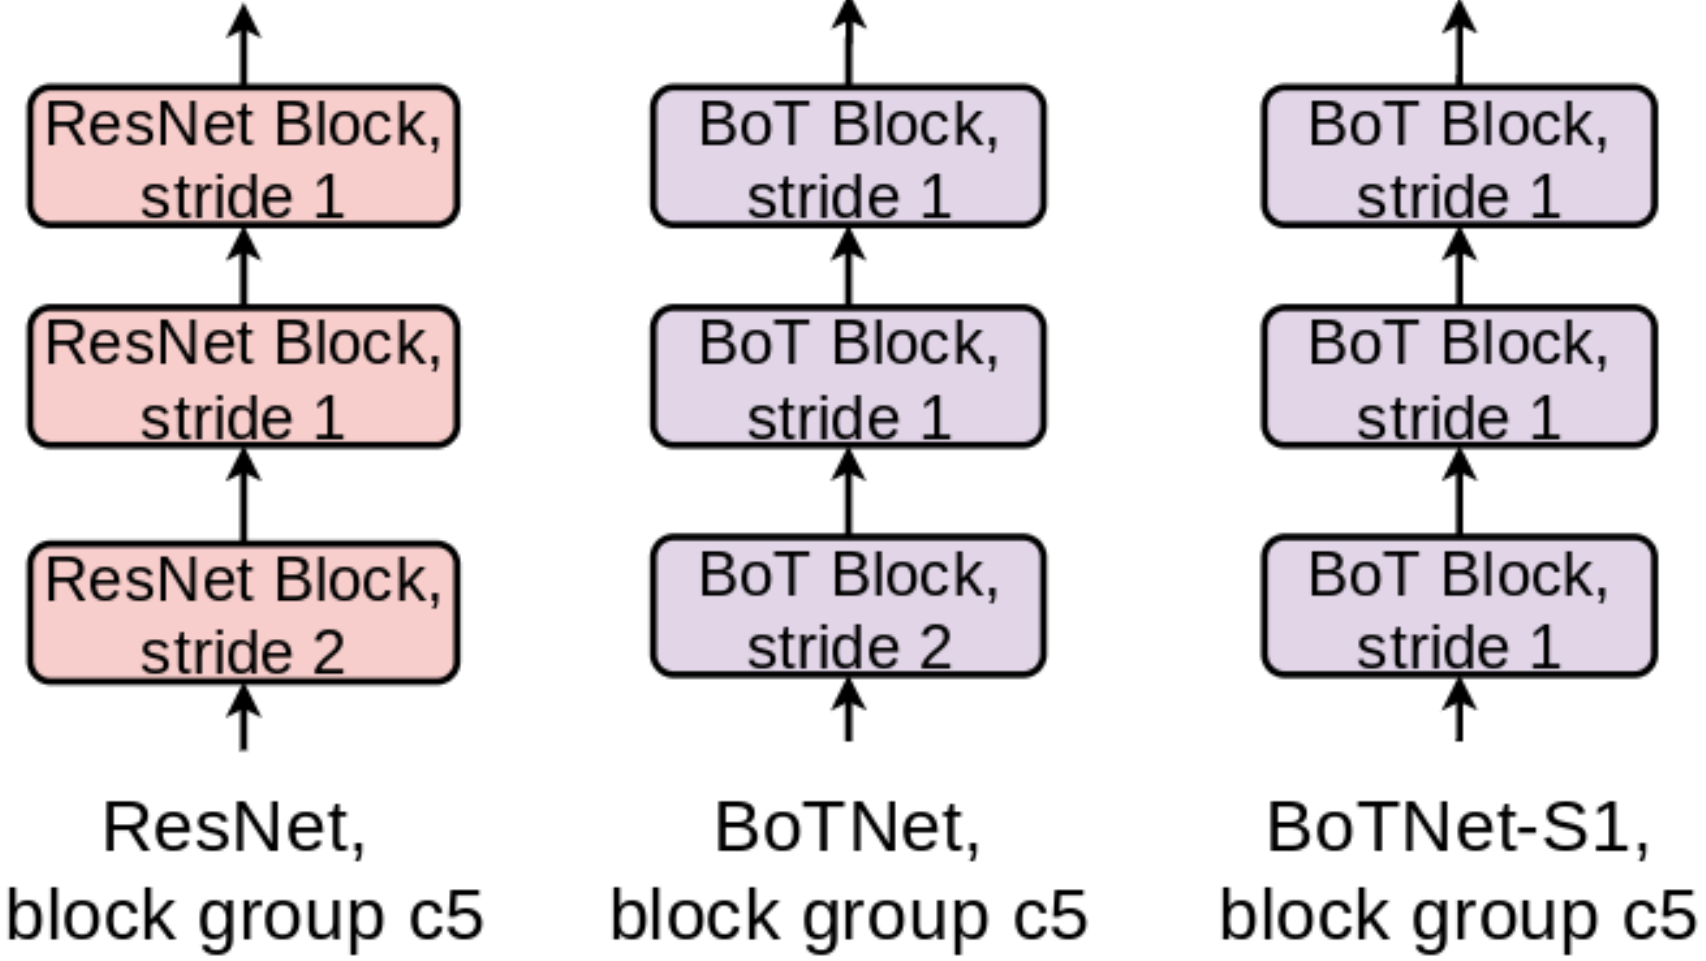}
    \caption{The \texttt{c5} (final) block groups for ResNet (left), BoTNet (middle) and BoTNet-S1 (right).}%
    \label{fig:s1}%
\end{figure}

\subsection{Non-Local Comparison}

The main paper offered a comparison between Non-Local Nets and BoTNets as well as an implementation of BoT blocks in the design of Non-Local Nets. In order to make it more clear visually, we provide an illustration of all designs in Figure \ref{fig:nonlocal_comp}. The figure clearly highlights the differences between inserting blocks vs replacing blocks. We note that the NL style insertion requires careful placement as prescribed in the original paper. On the other hand, simply replacing the final three blocks is a convenient design choice. Nevertheless, BoT blocks are still an improvement over vanilla NL blocks even in the insertion design, likely due to using multiple heads, relative position encodings, and value projection. As already explained in the main paper, even the {\it replacement} design of BoTNet performs better than the {\it insertion} design of vanilla NL, likely due to performing more self-attention (three vs one). Adding value projections to the NL block only improved the performance by 0.2 \apbbox{}, while the gains from using 4 heads in the MHSA layer in BoT block only helps by \~0.2\apmask{}. Therefore, BoT blocks can be viewed as an improved implementation of NL blocks with relative position encodings being the main driver of the performance difference.

\begin{figure}[ht]
\centering
\includegraphics[scale=.42]{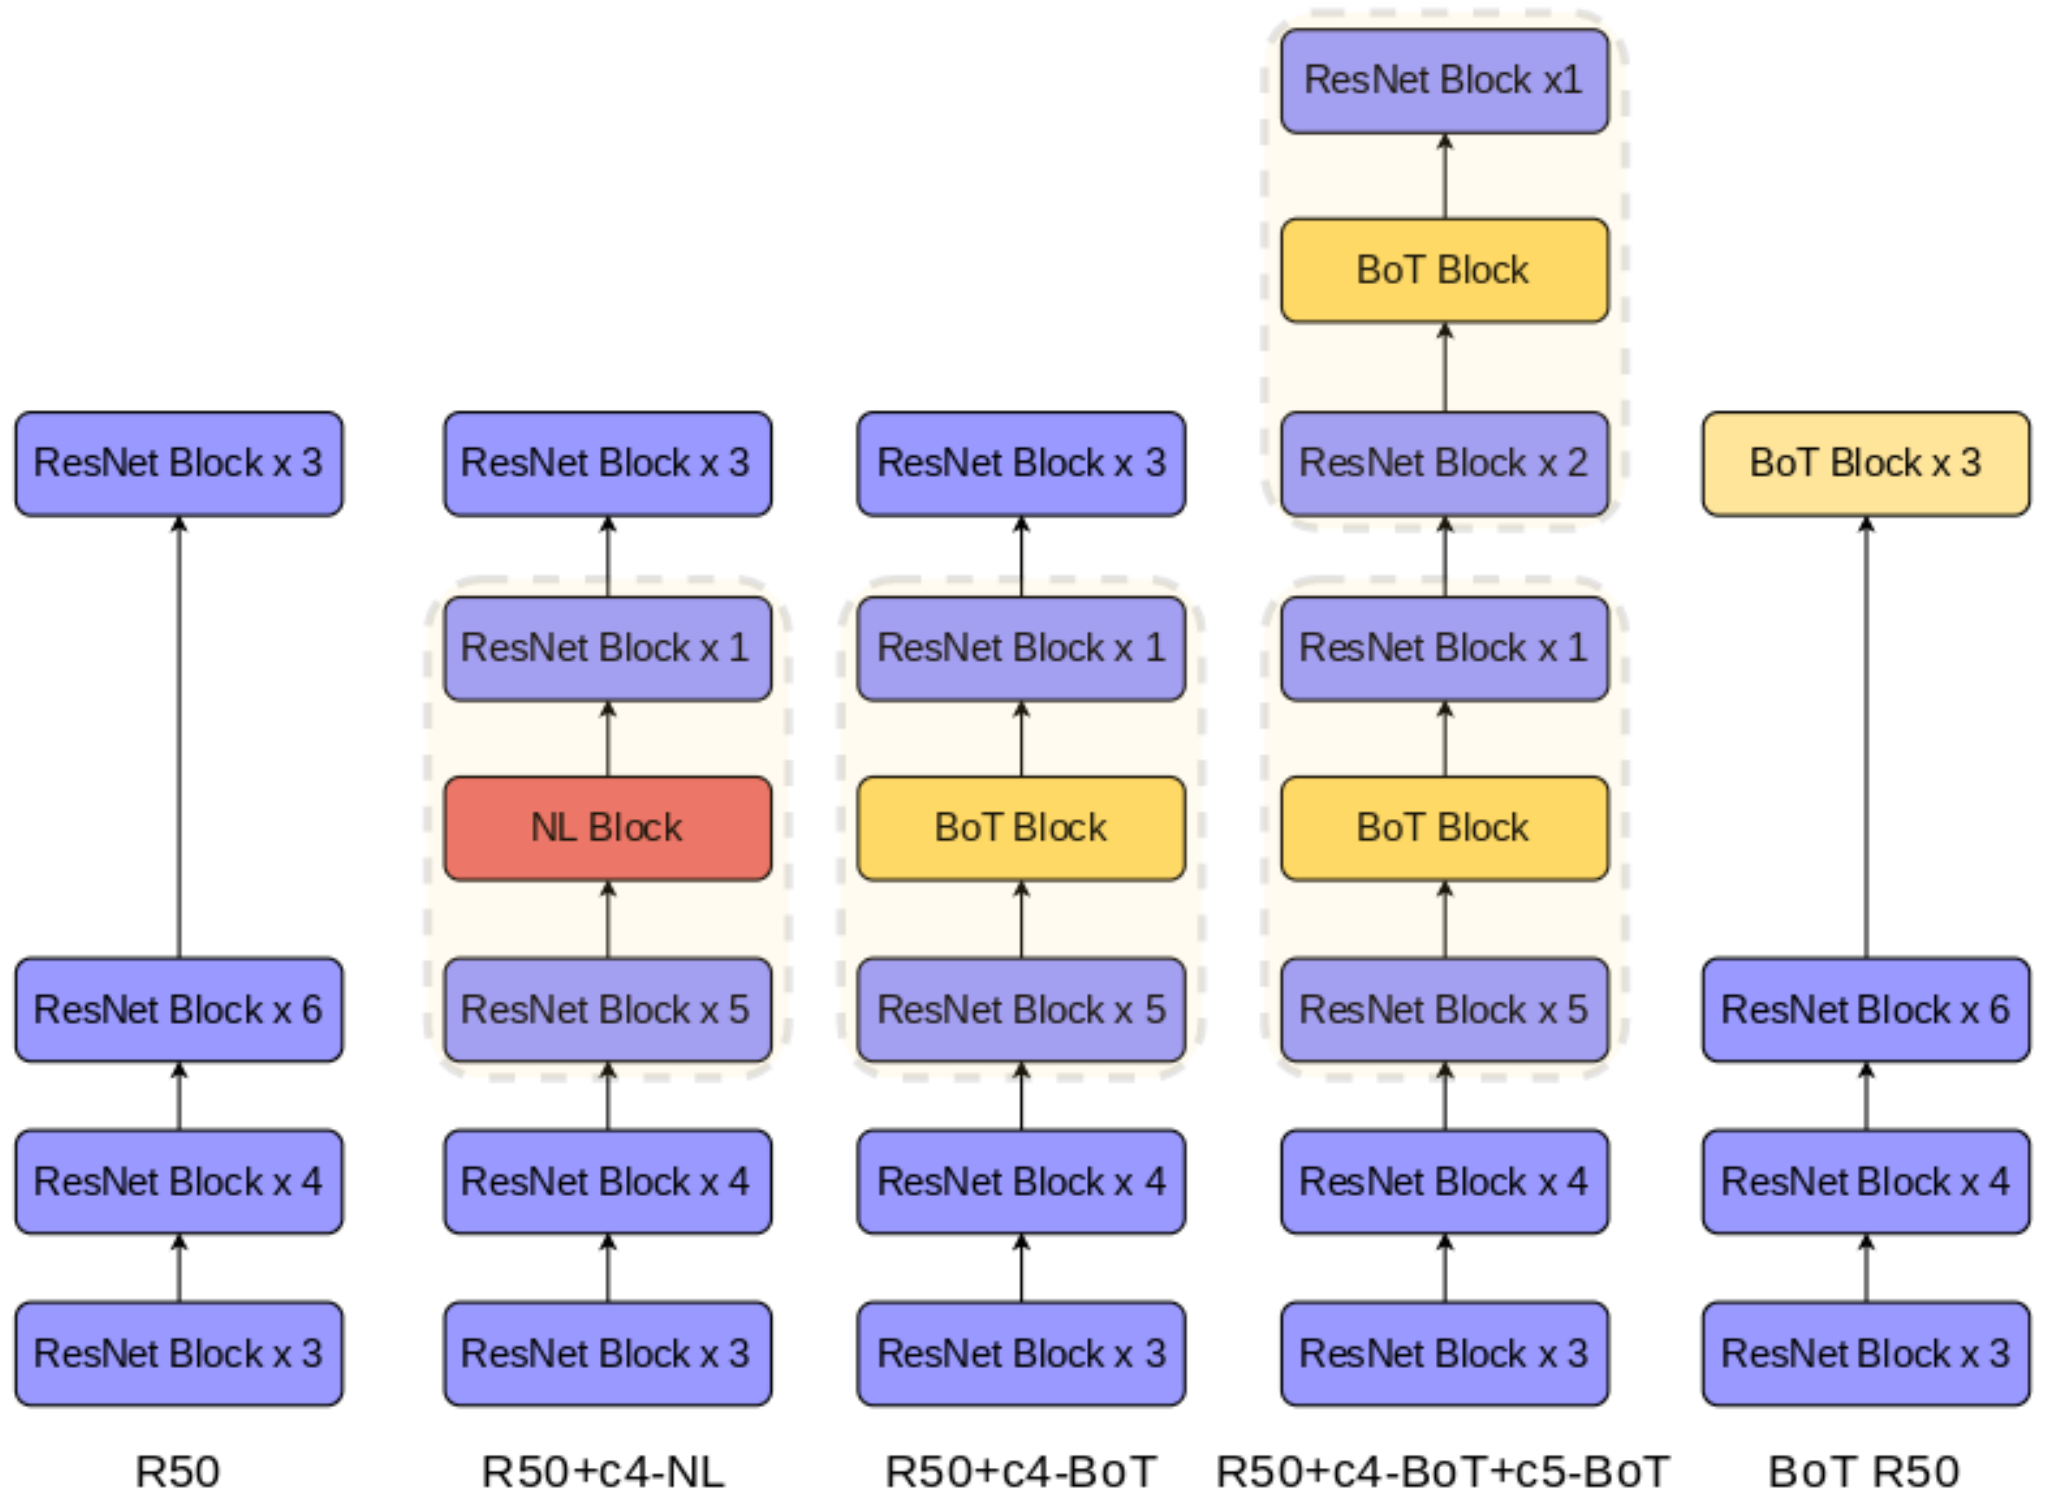}

\caption{{\bf First:} Regular ResNet 50 with \texttt{[3,4,6,3]} blockgroup structure. {\bf Second:} Non-Local (NL) block {\it inserted} in the \texttt{c4} blockgroup of a ResNet, between the pre-final and final ResNet block, as specificed by Wang et. al~\cite{wang2018non}. {\bf Third:} BoT block {\it inserted} in the same manner as a NL block with the differences between a BoT and NL block highlighted in in the main paper. {\bf Fourth:} 2 BoT blocks, one each in \texttt{c4,c5} blockgroups {\it inserted} in the same manner (between pre-final and final block) as prescribed by Wang et al.~\cite{wang2018non}. {\bf Fifth:} BoT50, where the final three ResNet blocks are {\it replaced} by BoT blocks.}
\label{fig:nonlocal_comp}
\end{figure}

\subsection{Comparison to Squeeze-Excite}

One may argue that squeeze-excitation blocks and self-attention blocks are very much related in the sense that both of them perform global aggregation and provide that as a context to convolutional models. Therefore, it is natural to ask for a comparison between the two blocks especially given that Squeeze-Excite (SE) blocks are computationally cheap and easy to use compared to BoT blocks. Table \ref{tab:squeeze_excite} presents this comparison. For fair comparison to BoTNet, we only place SE blocks in \texttt{c5} blockgroup and call this setup as R50+ c5-SE. We do not see any difference between R50 and R50 + c5-SE. However, we note that it is possible to get visible gains on top of R50 when placing SE blocks in all bottleneck blocks throughout the ResNet and not just in \texttt{c5}. Such a change (using SE in \texttt{c2,c3,c4}) is orthogonal to BoTNet and can be combined with BoTNet by using BoT blocks in \texttt{c5} and SE blocks in \texttt{c2,c3,c4}. We leave exploration of such architectures for future work.

\begin{table}[ht]\centering
\small
\setlength\tabcolsep{2.0pt}
\begin{tabular}{l|c|c}
\Xhline{1.0pt}
% \toprule
\text{Backbone}  & {\apbbox{}}  & {\apmask{}} \\[2pt]
\Xhline{1.0pt}

R50	& 42.1 & 	37.7  \\
BoT50 &	43.6 (\textcolor{ForestGreen}{+ {\bf 1.5}}) &	38.9 (\textcolor{ForestGreen}{+ {\bf 1.2}})  \\
R50 + c5-SE & 42.1 & 37.6 (- 0.1) \\
\hline

 \hline

 \Xhline{1.0pt}
 \end{tabular}
 \vspace*{-0mm}
 \caption{Comparing R50, BoT50 and R50 + c5-SE; all 3 setups using the canonical training schedule of 36 epochs, $1024\times 1024$ images, multi-scale jitter $\left[0.8, 1.25\right]$.}
 \label{tab:squeeze_excite}
 \vspace{-2mm}
 \end{table}

\subsection{ImageNet Test-Set Accuracy}

As has been the convention since 2017, our results in the paper only report and compare the validation set (50K images) accuracy on the ImageNet benchmark. However, the EfficientNet paper~\cite{tan2019efficientnet} presented updated results on the ImageNet test-set (100K images submitted on \url{http://image-net.org}). We also provide the results on the ImageNet test set for the ablation setup in Table \ref{tab:imresults_improved_further}, to verify that there are not any surprising differences between the validation and test set (Table \ref{tab:imresults_improved_further_test} presents similar numbers to Table \ref{tab:imresults_improved_further}). 

\begin{table}[ht]\centering
 \small
 \setlength\tabcolsep{1.0pt}
 \begin{tabular}{l|c}
 \Xhline{1.0pt}
\text{Backbone}  & {top-1 acc.}  \\[2pt]
\Xhline{1.0pt}

SE50 & 	79.3 \\
BoT-S1-50 &	80.3 (\textcolor{ForestGreen}{+ {\bf 1.0}})\\

\Xhline{1.0pt}
\end{tabular}
\vspace*{-0mm}
\caption{ImageNet {\it test set} results in a further improved training setting with SE blocks and SiLU non-linearity: 200 epochs, batch size 4096, weight decay 4e-5, RandAugment (2 layers, magnitude 10), and label smoothing of 0.1. R50 with SE blocks is referred to as SE50.}
\label{tab:imresults_improved_further_test}
\vspace{-2mm}
\end{table}

\subsection{Resolution Dependency in BoTNet}

Architectures such as BoTNet and ViT that use self-attention end up adopting position encodings~\cite{vaswani2017attention}. This in turn creates a dependency at inference time to use the same resolution that the model was trained for. For example, taking T7 trained at $384 \times 384$, and running inference with a different resolution (say $512 \times 512$) would introduce additional positional encodings. Purely convolutional architectures such as ResNets and SENets do not face this problem. We leave it for future work to investigate various design choices in making Transformer based architectures for vision, resolution independent at inference time. Some potential ideas are multi-resolution training with bilinearly interpolated positional encodings, using a spatial convolution before every self-attention operation (which could be performed without any positional encoding), etc.

While BoTNet-like hybrid architectures benefit from the spatial dependencies implicitly learned by the convolutional stack prior to attention, the reason we still use position encodings is because of the improvements that arise from using them. We also observe similar performance gains on the ImageNet benchmark. Using no position encoding at all for the BoT blocks still provides a gain of + 0.7\% top-1 accuracy, but lags behind the gains from using position encodings (+ 1.2\%). Further, relative position encoding is not as important in ImageNet benchmark as it is in the COCO benchmark. Absolute position encodings provide similar gains to relative posiition encodings. We believe this is likely due to the nature of the task being less contextual (and doesn't involve precise localization) for image classification compared to detection and segmentation. We retain relative position encodings for the ImageNet experiments for consistency with the architecture used for COCO. However, for practitioners, we recommend using absolute position encodings for image classification, especially when using convolutions prior to attention, since it is faster (for training and inference) and simpler to implement.

\begin{table}[ht]\centering
 \small
 \setlength\tabcolsep{1.0pt}
 \begin{tabular}{l|c|c}
 \Xhline{1.0pt}
\text{Backbone}  & Pos-Enc & {top-1 acc.}  \\[2pt]
\Xhline{1.0pt}

SE50 & N/A &	79.2 \\
BoT-S1-50 &	 - & 79.9 (\textcolor{ForestGreen}{+ {\bf 0.7}})\\
BoT-S1-50 &	 Abs & 80.2 (\textcolor{ForestGreen}{+ {\bf 1.0}})\\
BoT-S1-50 &	 Rel & 80.4 (\textcolor{ForestGreen}{+ {\bf 1.2}})\\

\Xhline{1.0pt}
\end{tabular}
\vspace*{-0mm}
\caption{ImageNet (val) results in a further improved training setting with SE blocks and SiLU non-linearity: 200 epochs, batch size 4096, weight decay 4e-5, RandAugment (2 layers, magnitude 10), and label smoothing of 0.1. R50 with SE blocks is referred to as SE50.}
\label{tab:posenc_imnet}
\vspace{-2mm}
\end{table}

\section{BoTNet and SENet Block Configs}

Please refer to Table \ref{tab:blockgroups} for block configs. of the various BoTNets and SENets used for the ImageNet experiments.

\begin{table}[ht]\centering
\small
\setlength\tabcolsep{2.0pt}
\begin{tabular}{l|c}
\Xhline{1.0pt}
% \toprule
\text{Model} & \text{Block Groups}  \\[2pt]
\Xhline{1.0pt}

ResNet-50 & \texttt{[3,4,6,3]} \\
ResNet-101 & \texttt{[3,4,23,3]} \\
ResNet-152 & \texttt{[3,8,36,3]} \\
\hline
SENet-50 & \texttt{[3,4,6,3]} \\
SENet-101 & \texttt{[3,4,23,3]} \\
SENet-152 & \texttt{[3,8,36,3]} \\
{SENet-350} & \texttt{[4,40,60,12]} \\
\hline
{BoTNet-S1-59} & \texttt{[3,4,6,6]} \\
{BoTNet-S1-77} & \texttt{[3,4,6,12]} \\
{BoTNet-S1-110} & \texttt{[3,4,23,6]} \\
{BoTNet-S1-128} & \texttt{[3,4,23,12]} \\

\Xhline{1.0pt}
\end{tabular}
\vspace*{-0mm}
\caption{Backbones and their block group configurations. All of them use the standard convolutional stem of the ResNet~\cite{he2016deep}. \texttt{[3,4,6,6]}, refers to the use of 3, 4, 6 and 6 blocks respectively in stages \texttt{c2,c3,c4,c5}. For BoTNet-S1 design, the final blockgroup \texttt{c5} uses a stride of 1 for all blocks. In order to reflect the improved training setting used in EfficientNets, the four BoTNet models (above) make use of SE blocks for blocks in the groups \texttt{c2,c3,c4}.}
\label{tab:blockgroups}
\vspace{-2mm}
\end{table}

\begin{table*}[ht]\centering
\small
\setlength\tabcolsep{2.0pt}
\begin{tabular}{l|c|c|cc|cc|c}
\Xhline{1.0pt}
% \toprule
\text{Model}  & \text{Backbone} & \text{Resolution} & \text{Top-1 Acc.}  & \text{Top-5 Acc.} & \text{Params} & \text{M.Adds} & \text{Steptime} \\[2pt]
\Xhline{1.0pt}

B0 & EfficientNet & 224 & 77.1 & 93.3 & 5.3M & 0.39B & 35.6 \\
{\bf S0} & {\bf SENet-50} & {\bf 160} & {\bf 77.0} & {\bf 93.5} & {\bf 28.02M} & {\bf 2.09B} & {\bf 32.3} \\
\hline

{\bf B1} & {\bf EfficientNet} & {\bf 240} & {\bf 79.1} & {\bf 94.4} & {\bf 7.8M} & {\bf 0.7B} &  {\bf 58.8} \\
- & ResNet-50 & 224 & 78.3 & 94.3 & 25.5M & 4.09B & 50.7 \\
- & ResNet-50 & 256 & 78.8 & 94.5   & 25.5M & 5.34B & 62.1 \\
- & SENet-50 & 224 & 79.4 & 94.6 & 28.02M & 4.09B & 64.3 \\
\hline

B2 & EfficientNet & 260 &  80.1 & 94.9 & 9.2M & 1.0B &  74.6 \\
- & {\bf ResNet-101} & {\bf 224} & {\bf 80.0} & {\bf 95.0} & {\bf 44.4M}  & {\bf 7.8B} & {\bf 63.0} \\
\hline

B3 & EfficientNet & 300 & 81.6 & 95.7 & 12M & 1.8B &  120.8 \\
T3 & BoTNet-S1-59 & 224 & 81.7 & 95.8 & 33.5M & 7.3B & 156.2 \\
- & ResNet-152 & 224 & 81.3 & 95.5 & 60.04M & 11.5B & 85.6 \\ 
{\bf S1} & {\bf SENet-101} & {\bf 224} & {\bf 81.4} & {\bf 95.7} & {\bf 49.2M} & {\bf 7.8B} & {\bf 71.1} \\
{\bf S2} & {\bf SENet-152} & {\bf 224} & {\bf 82.2} & {\bf 95.9} & {\bf 66.6M} & {\bf 11.5B}  & {\bf 97.7} \\

\hline

B4 & EfficientNet & 380 & 82.9 & 96.4 & 19M & 4.2B &  238.9 \\
{T4} & { BoTNet-S1-110} & {224} & {\bf 82.8} & {96.3} & {54.7M} & {10.9B} & {181.3} \\
{\bf S3} & {\bf SENet-152} & {\bf 288} & {\bf 83.1} & {\bf 96.4} & {\bf 66.6M} & {\bf 19.04B} & {\bf 149.9} \\

\hline
\hline

B5 & EfficientNet & 456 & 83.6 & 96.7 & 30M & 9.9B &  442.6 \\
S4 & SENet-350 & {320} & 83.6  & 96.6 & 115.18M & 52.9B & 397.9  \\ 
{\bf T5} & {\bf BoTNet-S1-128} & {\bf 256} & {\bf 83.5} & {\bf 96.5} & {\bf 75.1M} & {\bf 19.3B} & {\bf 355.2} \\
\hline

B6 & EfficientNet & 528 & 84.0 & 96.8 & 43M & 19B &  776.3 \\
S5 & SENet-350 & {384} & 83.8 & 96.6 & 115.18M & 52.9B & 397.9  \\ 
{\bf T6} & {\bf BoTNet-S1-77} & {\bf 320} & {\bf 84.0} & {\bf 96.7} & {\bf 53.9M} & {\bf 23.3B} &  {\bf 578.1} \\

\hline
B7 & EfficientNet & 600 &  84.3 & 97.0 & 66M & 37B &  1478.4 \\
{\bf T7-320} & {\bf BoTNet-S1-128} & {\bf 320} & {\bf 84.2} & {\bf 96.9} & {\bf 75.1M} & {\bf 30.9B} & {\bf 634.3} \\
B7-RA & EfficientNet & 600 & 84.7 & 97.0 & 66M & 37B &  1478.4 \\
{\bf T7} & {\bf BoTNet-S1-128} & {\bf 384} & {\bf 84.7} & {\bf 97.0} & {\bf 75.1M} & {\bf 45.8B}  & {\bf 804.5} \\

\hline
\Xhline{1.0pt}
\end{tabular}
\vspace*{-0mm}
\caption{Various backbone architectures, evaluated under the fair setting of using the improved training elements from EfficientNet~\cite{tan2019efficientnet}. Models are grouped by the accuracy of each EfficientNet model. For ResNets, SENets and BoTNets, the best weight decay from \texttt{[2e-5,4e-5,8e-5,1e-4]} the best dropconnect from \texttt{[0.2,None]}, and the best RandAugment magnitude from \texttt{[9,15,24]} are used to ensure fair comparisons to the already well tuned EfficientNets whose results we take from the latest update to the official codebase. The steptimes that we report, refer to the {\bf {compute}} time on a TPU-v3 core, for a batch size of 32 for all the models. This is to ensure we do not use different batch sizes for different models and do not conflate TPU rematerialization for dense convolutions. Had we done so (i.e picked bigger batch sizes for ResNets and BoTNets as long as they fit on memory), the speedup gains would be even higher. Further, by {\bf compute} time, we just mean the time spent for forward and backward passes, and {\bf not} the data loading. This is again to ensure comparisons across models do not exploit inefficient (or non-cached) data loading. B7-RA refers to EfficientNet-B7 trained with RandAugment~\cite{cubuk2020randaugment}.}
\label{tab:backbones_all}
\vspace{-2mm}
\end{table*}

\subsection{Hyperparameters}

Please refer to Table \ref{tab:hparams_all} for the hyperparameters used for all backbones presented for ImageNet classification results in Table \ref{tab:backbones_all}.

\begin{table*}[ht]\centering
\small
\setlength\tabcolsep{2.0pt}
\begin{tabular}{l|c|c|c|c|c|c}
\Xhline{1.0pt}
% \toprule
\text{Model}  & \text{Backbone} & \text{Resolution} & \text{WD}  & \text{RA} & \text{DC} & \text{DR} \\[2pt]
\Xhline{1.0pt}

{S0} & {SENet-50} & {160} & 8e-5  & 9 & 0.2 & 0.25\\
\hline

- & ResNet-50 & 224 & 8e-5  & 9 & - & - \\
- & ResNet-50 & 256 & 8e-5  & 9 & - & - \\
- & SENet-50 & 224 & 4e-5  & 15 & 0.2 & 0.25 \\
\hline

- & {ResNet-101} & {224} & 4e-5  & 15 & 0.2 & 0.25 \\
\hline

T3 & BoTNet-S1-59 & 224 & 4e-5  & 15 & 0.2 & 0.25 \\
- & ResNet-152 & 224 & 4e-5  & 15 & 0.2 & 0.25 \\ 
{S1} & {SENet-101} & {224} & 4e-5  & 15 & 0.2 & 0.25 \\
{S2} & {SENet-152} & {224} & 4e-5  & 15 & 0.2 & 0.25 \\

\hline

{T4} & { BoTNet-S1-110} & {224} & 4e-5  & 15 & 0.2 & 0.25 \\
{S3} & { SENet-152} & { 288} & 4e-5  & 15 & 0.2 & 0.25  \\

\hline

S4 & SENet-350 & {320} & 4e-5  & 15 & 0.2 & 0.25  \\ 
{T5} & {BoTNet-S1-128} & {256} &  4e-5  & 15 & 0.2 & 0.25 \\
\hline

S5 & SENet-350 & {384} & 4e-5  & 15 & 0.2 & 0.25  \\ 
{T6} & {BoTNet-S1-77} & {320} &  4e-5 &  15 & 0.2 & 0.25 \\

\hline
{T7-320} & {BoTNet-S1-128} & 320 & 2e-5 & 24 & 0.2 & 0.25  \\
{T7} & {BoTNet-S1-128} & 384 & 2e-5 & 24 & 0.2 & 0.25  \\

\hline
\Xhline{1.0pt}
\end{tabular}
\vspace*{-0mm}
\caption{Hyperparameters for ResNets, SENets and BoTNets trained for ImageNet-1K classification benchmark reported in Table \ref{tab:backbones_all}. Resolution, WD, RA, DC and DR refer to image size, weight-decay, randaugment magnitude (2 layers), dropconnect probability and dropout ratio respectively. Our implementation of drop-connect and the balance between RA and WD is similar to HaloNets~\cite{vaswani2021halo}. Numbers reported for EfficientNet are just taken from the EfficientNet paper~\cite{tan2019efficientnet}. All models additionally use label smoothing of $0.1$ and trained for 350 epochs. All models are trained with global batch size $4096$, trained on TPU v3 hardware (v3-128), and {\it no} synchronized (cross-replica) batch-norm was used for training any of these models, unlike EfficientNet. We expect results to improve marginally with the use of sync. batchnorm. Training uses \texttt{bfloat16} precision and the throughput speeds reported also use \texttt{bfloat16} precision. The evaluation for all models were run on TPU v3-8 hardware with global batch size of 128 using \texttt{bfloat16} precision. All models use SGD-momentum optimizer (without Nesterov) with a momentum of 0.9. The base learning rate is $0.1$ for a batch size of 256 as is standard, and is scaled to 1.6 for a batch size of 4096, with linear warmup for 5 epochs, and cosine decay for rest of the training. } 
\label{tab:hparams_all}
\vspace{-2mm}
\end{table*}

\subsection{M.Adds and Params}

In-built tools for computing parameters and FLOPs (2 * M.Adds) are often not accurate when used on architectures with \texttt{einsums}. We therefore explicitly calculated the M.Adds we report in this paper using this script \url{https://gist.github.com/aravindsrinivas/e8a9e33425e10ed0c69c1bf726b81495}.

\subsubsection{Effect of SE blocks, SiLU and lower weight decay}

Other aspects of improved training of backbone architectures for image classification has been the use of Squeeze-Excitation (SE) blocks~\cite{hu2018squeeze}, SiLU non-linearity~\cite{elfwing2018sigmoid, ramachandran2017searching, hendrycks2016gaussian} and further lowering the weight decay (for eg., EfficientNet uses 1e-5). When employing SE blocks in BoTNet and BoTNet-S1, we only do so for the ResNet blocks that employ $3\times 3$ convolutions since self-attention is already designed for contextual global pooling. As expected, these changes lead to further improvements in the accuracy for all the models, with the gains from BoTNet remaining intact over the baseline SENet (ResNet with SE blocks) (Table \ref{tab:imresults_improved_further}).

\begin{table}[ht]\centering
 \small
 \setlength\tabcolsep{1.0pt}
 \begin{tabular}{l|c|c}
 \Xhline{1.0pt}
\text{Backbone}  & {top-1 acc.} & {top-5 acc.} \\[2pt]
\Xhline{1.0pt}

SE50 & 	79.2 &	94.6 \\
BoT50 &	79.6 (\textcolor{ForestGreen}{+ {\bf 0.4}}) &	94.6 \\
BoT-S1-50 &	80.4 (\textcolor{ForestGreen}{+ {\bf 1.2}}) & 95.0 (\textcolor{ForestGreen}{+ {\bf 0.4}}) \\

\Xhline{1.0pt}
\end{tabular}
\vspace*{-0mm}
\caption{ImageNet results in a further improved training setting with SE blocks and SiLU non-linearity: 200 epochs, batch size 4096, weight decay 4e-5, RandAugment (2 layers, magnitude 10), and label smoothing of 0.1. R50 with SE blocks is referred to as SE50.}
\label{tab:imresults_improved_further}
\vspace{-2mm}
\end{table}

The improvements from Table \ref{tab:imresults_improved_further} suggest that BoTNets are a good replacement for ResNets and SENets, especially when trained with data augmentations and longer training schedules. We have also made sure to present strong baselines (eg. 79.2\% top-1 acc. SENet-50). 

\subsection{Discussion}
Figure \ref{fig:pareto} presents all the three model families (SENets, EfficientNets and BoTNets) together in one plot. %Please refer to Figures \ref{fig:pareto_resnet} and \ref{fig:pareto_botnet} for zoomed-in versions of the global figure. 
As discussed in the previous sections, SENets are powerful models with strong performance that is better than EfficientNets and can be scaled all the way up to 83.8\% top-1 accuracy without any bells and whistles such as ResNet-D, etc. BoTNets initially perform worse than SENets (\eg T3) but begin to take over in terms of performance from T4 and strictly outperform EfficientNets, especially towards the end. EfficientNets do not scale well, particularly in the larger accuracy regime. %This definitely suggests that the compound scaling rule in EfficientNets may not be strong enough and simple depth scaling (as in ResNet-RS~\cite{bello2021revisit}) works well enough. A more careful study of scaling rules for all these model classes is left for future research.

Recently, Transformer based models for visual recognition have become very popular since the Vision Transformer (ViT) model~\cite{dosovitskiy2020image}. While our paper was developed concurrently to ViT, there has been a lot of follow-up to ViT such as DeiT~\cite{touvron2021training} that have further improved the results of ViT on ImageNet-1K through regularization and distillation. As seen in the results and emphasized already, DeiT-384 is {outperformed} by both SENets and BoTNets currently when not considering distillation. This suggests that convolutional and hybrid (convolution and self-attention) models are still strong models to beat as far as the ImageNet benchmark goes. The message in ViT was that pure attention models without extra regularization struggle in the small data (ImageNet) regime\footnote{ImageNet-1K may not be a small dataset by conventional standards, but is referred to as such here for the contrast with JFT.}, but shine (achieve {\bf 85.1\%} and {\bf 88.6}\% fine-tuned top-1 accuracy) in the large data regime (ImageNet-21k and JFT dataset), where inductive biases such as data augmentation and regularization tricks used in the EfficientNet training setting are less important. Nevertheless, we think it is an interesting exercise to explore hybrid models such as BoTNet even in the large data regime simply because they seem to scale much better than SENets and EfficientNets (Figure \ref{fig:pareto}) and achieve better performance than DeiT on ImageNet. We leave such a large scale effort for future work. %It is also possible to design pure attention models that scale better than ViT in the large data regime, example, those employing local attention such as SASA~\cite{ramachandran2019stand}.

It is unclear what the right model class is, given that we have not yet explored the limits of hybrid models in the large data regimes, and that the pure attention models currently lag behind both convolutional and hybrid models in the small data regime. Nevertheless, with the hope that the ImageNet-1K benchmark has been representative of the best performing models in the vision community, BoTNets are likely to be a simple and compelling baseline to always consider. 
BoTNets are very much similar to the Hybrid-ViT models (R50 + ViT-B/16). The few minor differences have already been highlighted in the main paper, as to how BoTNets use Bottleneck Transformer (BoT) blocks, which are different from the regular Transformer blocks in ViT. These differences {\it may} lead to different optimizers and hyperparameters for training BoT and ViT models, e.g, SGD-momentum (BoT) \vs Adam (ViT); BatchNorm (BoT) \vs LayerNorm (ViT), number of non-linearities and residual connections, etc. One useful aspect of BoTNets is that they can exploit the hyperparameters that have been developed over many years for ResNets (SGD, BatchNorm, etc), resulting in a straightforward adoption in other vision tasks such as instance segmentation and object detection. These are benchmarks that have not yet seen widespread use of the Adam optimizer, LayerNorm and Transformer layers, yet. An appealing aspect of hybrid models in BoTNets over ViT-hybrids is their parameter and FLOPs efficiency. The ViT paper has not explicitly optimized for the design of hybrids. So, we believe strong conclusions cannot be drawn yet, and a careful empirical study of their differences is left for future work.

Our paper does not touch upon comparisons to backbones that employ group convolutions~\cite{xie2017aggregated, radosavovic2020designing}, concurrent work on channel (or linear) attention in \texttt{c4}~\cite{bello2021lambdanetworks}, axial attention~\cite{wang2020axial, shen2020global} and local attention~\cite{ramachandran2019stand}, but we remark that changes prior to the \texttt{c5} blockgroup can benefit BoTNets as well. We also leave it to future research to carefully compare alternatives to self-attention such as lambda-layers~\cite{bello2021lambdanetworks}. We speculate that employing local attention in earlier blockgroups such as \texttt{c2,c3,c4} with the SASA~\cite{ramachandran2019stand} layers could lead to more efficient pure attention models in future. Our paper is a contribution in terms of identifying connections between ResNet MHSA blocks, Transformer blocks, and Non-Local blocks; and showing the power of simple hybrids, to achieve SoTA-competitive backbone architecture performance on both COCO and ImageNet-1K benchmarks.

\end{appendix}
